# Supplementary material for: Single-shot Hyperspectral-Depth Imaging with Learned Diffractive Optics
Source: arXiv:2009.00463 source file (2021-08-15)
Supplement: Supplementary file 1 [file supplemental.tex]

\begin{figure*}[t]
  \centering
  \includegraphics[width=\linewidth]{figs/real_vs_fabricated_doe.pdf}%
  \vspace{-0mm}%
  \caption{\label{fig:real_vs_fabricated_doe}%
 (a) Our learned PSF shows depth and spectral dependency, allowing us to acquire both data from a single shot.
 (b) We calibrate the PSF of the fabricated DOE matched with the simulation counterpart. }
  \vspace{-3mm}
\end{figure*}

This document provides additional details and results.

\section{Network Architecture}
\label{sec:network}
For a given input image either generated by our wave-optics simulator or captured by our camera prototype, we reconstruct a hyperspectral image and a depth map using a convolutional neural network (CNN).
Figure~\ref{fig:network_full} shows our network architecture.
Our CNN architecture is inspired by a U-net \cite{ronneberger2015u} with the difference of using two decoders instead one.
The network takes a RGB sensor image as inputs.
During training, 256$\times$256 patches are fed through a basic block layer that consists of two pairs of a 3$\times$3 convolutional layer with batch normalization and PReLU. We use max pooling after each of this basic block to implement the encoder architecture.
The spatial resolution is reduced by half at each pooling stage and the number of channels is doubled.
We obtain the feature with 1024 channels after the encoder.
A counterpart decoder has the similar design with the encoder using a basic block at each spatial resolution and a transposed convolution for upscaling. We have skip connections from the encoders to the decoders at each resolution.
The final convolutional layers enable us to match the number of output channels to the hyperspectral image and the depth map.
For the spectral decoder, we added the spectrally upsampled image of to the output of the spectral decoder for residual learning.

\begin{figure*}[t]
  \centering
  \vspace{-2mm}
  \includegraphics[width=\linewidth]{figs/network_full.pdf}
  \vspace{-5mm}
  \caption{\label{fig:network_full}%
  {Reconstruction Network.} The input to the network is a sensor image with three channels (RGB).
  The single-encoder-dual-decoder architecture with skip connections enable us to reconstruct a depth map and a hyperspectral image of 25 channels from 420 to 660\,nm in 10\,nm intervals.
  For details of the spectral upsampling, we refer to the main paper.
  The top row shows the width and height of the patch sizes during training.
  We denote the number of channels in each layer, where the input and output channels are shown in the top and the bottom of each block.}
  \vspace{-2mm}
\end{figure*}

\begin{figure}[tph]
  \centering
  \includegraphics[width=0.9\linewidth]{figs/psf_fit_analysis.pdf}
  \vspace{-0mm}
  \caption{\label{fig:psf_fit_analysis}%
  {Analyzing the PSF of the prototype DOE.}
  (a-b) Due to the low diffraction efficiency of the DOE prototype, we have a low-frequency component in the PSF in addition to the intended high-frequency component.
  (c) For a row on the image, we plot the gradient values, revealing the high-frequency and the low-frequency components.}
  \vspace{-5mm}
\end{figure}

\section{Hyperspectral-Depth Dataset}
Our HS-D dataset has 16 indoor scenes.
Each scene has a triplet of a hyperspectral image, a depth map, and a background mask with pixel-accurate alignment.
The hyperspectral image is in reflectance domain, making it effective for spectral augmentation as shown in the main paper.
Spectral range starts from $420$ to $680$\,nm in $10$\,nm intervals, resulting in $27$ spectral channels.
The depth map has accurate values ranging from $0.4$ to $2.0$\,m obtained by a structured light scanning.
The background mask for invalid spectral and depth regions is also provided for selectively choosing valid patches for training.
Every image has the spatial resolution of $2824\times4240$.

\mparagraph{Data augmentation for HS-D training}
We augment our HS-D dataset for robust learning.
First, we spatially scale the images with the factors of 0.25, 0.50, and 1.00.
We use bilinear interpolation for hyperspectral images and nearest-neighbor interpolation for depth maps and background masks.
Second, we augment depth maps by globally translating the depth values along the $z$-axis by -0.2\,m, 0.0\,m, and 0.2\,m.
Third, we spectrally augment the dataset by multiplying the hyperspectral reflectance images with 29 different CIE standard illuminants, yielding radiance maps under various illuminations.
In total, we have $\sim$20,000 patches.

\mparagraph{Benchtop combinational system for dataset acquisition}
We build a benchtop combinational imaging system to capture our HS-D dataset.
We use a projector (EPSON EB-X31) and a liquid-crystal-tunable-filter hyperspectral camera which consists of a machine vision camera (Pointgrey GS3-U3-91S6M-C), a liquid crystal tunable filter (VariSpec LCTF VIS), a relay lens (Sigma A, $f$/1.4, 50\,mm), a collimating lens (Sigma A, $f$/1.4, 50\,mm), and an imaging lens (Nikon, $f$/2.0, 35\,mm).
To capture each scene, we illuminate it with a solid-state plasma light source (Thorlabs HPLS-30-4) and capture spectral images with the f-number of 22 from 420\,nm to 700\,nm by the LCTF modulation.
We capture and average the five spectral images for the low wavelengths (420\,nm to 450\,nm) to mitigate noise.
We then turn off the plasma light source and sequentially illuminate the scene with the gray-code patterns using the projector and capture the images with the point gray camera.
The LCTF is set to 600\,nm for the structured-light capture.

\mparagraph{HS-D dataset from raw captures}
We obtain dark-level images of the hyperspectral camera by capturing spectral images while blocking incident light to the lens.
We subtract the dark levels from every raw capture and denoise it with 3$\times$3 median filtering.
In each scene, we have a standard reflectance tile (Spectralon) that provides the calibrated illumination spectrum incident to the scene.
We use this measurement to obtain reflectance images.

We estimate depth maps using triangulation from the gray-coded inputs~\cite{moreno2012simple}.
Note that the structured-light scanning often provide inaccurate reconstruction for image regions with low albedo.
Therefore, we manually mask the black background out and apply depth refinement for the foreground objects~\cite{levin2007image}, resulting in a dense depth map for each scene.
The spatial resolution of each hyperspectral-depth image is 2824$\times$4240.

\mparagraph{Preprocessing for training and testing}
We divide 18 scenes into 13 scenes for training and 5 for testing.
We then collect 256$\times$256-sized HS-D patches.
Background dominant patches having invalid depth values or too low intensity are excluded for both training and testing.
We also ensured that only one of the 13 training scenes includes a ColorChecker in a set of training minibatches in order to avoid overfitting to this target.

\section{HS-D Encoded PSF}
Our learned PSF changes its shape for spectrum and depth.
Figure~\ref{fig:real_vs_fabricated_doe} shows the spectral-depth dependency of the simulated PSF as well as the calibrated PSF obtained from our prototype DOE.

\mparagraph{Calibration}
\label{sec:psf-calibration}
We calibrate the PSF for a combination of depth values and spectrum.
To this end, we use a solid-state plasma light source (Thorlabs HPLS-30-04) covered with a high-power precision pinhole (Thorlabs P23C) with a 25\,$\mu$m aperture.
In a dark room, we place the illumination module at target distances from $\sim$0.4 to 2.0\,m.
We apply spectral filtering in front of the camera using a Varispec LCTF filter in 10\,nm intervals and captured HDR hyperspectral images at each depth.
We also calibrate the spectral response function of the Canon Mark III camera by measuring its response to the calibrated light source~\cite{baek2017compact}.

\mparagraph{Diffraction efficiency}
Prototype DOEs typically present a low-frequency component in its PSF as zeroth-order diffraction, due to the low diffraction efficiency~\cite{peng2016diffractive,jeon2019compact}.
We examine the frequency response of our DOE prototype by capturing a black-white scene (Figure~\ref{fig:psf_fit_analysis}).
As expected, our PSF consists of two-frequency components: one with high frequency and the other with low frequency, where each can be modeled as a Gaussian function of mean (1445/10.74) and standard deviation (1458/312.27) in pixels.
We attempt to mitigate such low-frequency degradation of the captured images as detailed in Section~\ref{sec:e2e_opt}.

\section{Details on Hyperspectral Comparison}
With consideration of computational resource and algorithms performance, we adjusted the spatial resolution of experiments. For Jeon et al.~\cite{jeon2019compact} and ours, we use the half resolution of the test images in 1412-by-2120. For Baek et al.~\cite{baek2017compact}, we reduce the resolution of the input image by one-eighth as their method takes about 45\,minutes to process a 353-by-530 hyperspectral image.

\section{Details on Depth Comparison}
We compared our approach to two other DOE-based depth imaging methods: Wu et al.~\cite{wu2019phasecam3d} and (c) Chang et al.~\cite{Chang:2019:DeepOptics3D}.
The experimental configurations of these three methods are different including the effective pixel pitch, aperture diameter, the network design, the training dataset, and the camera response function.
We implemented a PSF simulator for Chang et
al.~\cite{Chang:2019:DeepOptics3D} and simulated PSFs with the same configuration of our prototype.
For Wu et
al.~\cite{wu2019phasecam3d}, we obtained the PSFs using the author-provided DOE height map that assumes the pixel pitch of 4.29\,um and the aperture size of 0.8\,mm.
The simulated PSFs are shown in the main paper demonstrating that the simulated PSF shapes match those reported in the original works.
Our U-net-based reconstruction network was used to train all DOE designs on our HS-D dataset.
Note that the spectral decoder was deactivated in this experiment. %

\section{DOE initialization}
Jointly optimizing a DOE and a CNN for hyperspectral-depth imaging is a challenging, non-convex inverse problem that aims at simultaneously solving multiple traditional problems, including phase retrieval, spectral super-resolution, monocular depth estimation, and deconvolution.
This non-convex nature makes it crucial to find a good initialization of the optimization parameters.
In particular, the initialization of the DOE has been shown to be important and is specific to a target application~\cite{wu2019phasecam3d}.
For hyperspectral-depth imaging, we therefore seek to find a proper initialization of the DOE through a Fisher-information-based optimization to obtain the initial DOE height field~\cite{shechtman2014optimal}.
Since the Fisher information matrix for the general hyperspectral depth imaging problem is too large to evaluate, we consider a simpler subproblem where we estimate the location and wavelength of a monochromatic point-source emitter from its single RGB image (${J}_{c}$).
Its Fisher information matrix $\mathcal{I}$ then describes the sensitivity of  the observed PSF to the spatial emitter positions ($p_x$, $p_y$, $p_z$) and wavelengths ($p_\lambda$).
When the brightness of the point source is known, the Fisher information matrix under the Gaussian noise model is given as:
\begin{equation}\label{eq:fisher_mat}
{\mathcal{I}_{ij}}\left( {\mathbf{\delta }} \right) = \sum\limits_{c, k} {\frac{1}{{\sigma^2 }}\frac{{\partial {{J}_{c}}\left( k; \delta, h \right)}}{{\partial {{\mathbf{\delta }}_i}}}\frac{{\partial {{J}_{c}}\left( k; \delta, h \right)}}{{\partial {{\mathbf{\delta }}_j}}}},
\end{equation}
where $\mathbf{\delta}=\{p_x,p_y,p_z,p_\lambda\}$, $\sigma$ is the standard deviation of the Gaussian noise, $k$ is the pixel index, and $h$ is the DOE height field.
While the Fisher information depends on the position and wavelength of the point-source emitter, we aim to find a DOE height field that provides high Fisher information for all sources in our design space.
To achieve this, we optimize the height of the DOE by minimizing the mean of the $A$-optimality of the Fisher information matrix over a set of monochromatic point sources located on the optical axis:
\begin{equation}\label{eq:fisher_opt}
\mathop {{\rm{minimize}}}\limits_h \frac{1}{N} \sum\limits_{p_\lambda  \in {\bf{\Lambda }}} {\sum\limits_{p_z \in {\bf{z}}} {{\mathcal{A}}\left( {p_z, p_\lambda ;h } \right)} },
\end{equation}
where ${\mathcal{A}}$ is the $A$-optimality, which is the trace of the inverse of the Fisher information matrix~$\mathcal{I}$.
The design space of the imaging system is characterized by the set of wavelengths $\bf{\Lambda}$ and the set of the depth layers $\bf{z}$ where the point sources are placed.
Since Equation~\eqref{eq:fisher_opt} is not a convex problem, we solve it based on stochastic gradient descent optimization, using the Adam optimizer.
This optimization itself requires an initialization, for which we choose a conventional Fresnel DOE lens pattern.
We set the brightness of the point source so as to ensure the maximum intensity of the captured PSFs of a Fresnel lens is $0.8$ of the maximum intensity of the image.

\mparagraph{Evaluation}
We tested three different initial DOE designs for end-to-end HS-D imaging: the Fresnel lens, the spiral DOE~\cite{jeon2019compact}, and the Fisher-information-based DOE.
Table~\ref{tab:init_psfs} compares how much the end-to-end optimization process of optics improves the accuracy of reconstructed spectral and depth information for different initializations.
Among the three candidates, we chose the Fisher-based initialization as it is superior to other initializations in terms of spectral and depth accuracy.

\begin{table}[hpbt]
\resizebox{\columnwidth}{!}{
\begin{tabular}{c|c|c|c|c}\hline
\multicolumn{2}{c|} {Initialization} & Fresnel & Spiral~\cite{jeon2019compact} & Fisher~\cite{shechtman2014optimal} \\ \hline \hline
\multirow{2}{3mm}{\begin{sideways}{\small{Spec.}}\end{sideways}}
& PSNR {[}dB{]} & 27.96$\rightarrow$28.68  & 26.90$\rightarrow$27.67 & 28.51$\rightarrow$\textbf{29.31} \\
& SSIM  & 0.74$\rightarrow$0.78  & 0.64$\rightarrow$0.75  &   0.79$\rightarrow$\textbf{0.81} \\ \hline
\multirow{2}{3mm}{\begin{sideways}{\small{Depth}}\end{sideways}}
& RMSE {[}m{]} &  0.21$\rightarrow$\textbf{0.19} &  0.32 $\rightarrow$ 0.26 &  0.23 $\rightarrow$ {0.20}  \\
& MAE {[}m{]} & 0.15 $\rightarrow$ 0.12  &  0.20 $\rightarrow$ 0.18 &  0.15 $\rightarrow$ \textbf{0.12} \\ \hline
\end{tabular}}
\caption{\label{tab:init_psfs}%
  {DOE initialization for end-to-end learning.}
  We used three different DOE initializations for our end-to-end optimization.
 The Fisher-initialized DOE optimization is superior to other initializations for spectral and depth reconstruction, and the Fresnel-lens-initialized optimization is the second best option.}
\end{table}
